# Supplementary material for: Spin-Selective Electron Transport Through Single Chiral Molecules
Source: arXiv:2309.07588 ancillary file (2023-09-14)
Supplement: Supplementary file 1 [file SI_Transport.pdf]

Supporting Information

# Spin-Selective Electron Transport Through Single Chiral Molecules

*M.R. Safari*, F. Matthes, C.M. Schneider, K.-H. Ernst*, D.E. Bürgler**

## CONTENTS

S1. Experimental Procedures S3

A. Molecule Synthesis S3

B. Sample Preparation S3

C. STM/STS Measurements S3

S2. Magnetic Sensitivity of the STM Tip S6

S3. Single-Molecule $I - V$ Spectra S7

S4. Reversing the Magnetization Direction of the STM Tip S9

References S10

## S1. EXPERIMENTAL PROCEDURES

All measurements were carried out in a multi-chamber UHV system with a base pressure of $< 10^{-8}$ Pa comprising a substrate preparation and analysis chamber, a distinct chamber for the controlled deposition of molecules, and a low-temperature scanning tunneling microscope (LT-STM from Omicron Scienta) operating at a temperature of 5 K.

### A. Molecule Synthesis

The synthesis of racemic mixtures of heptahelicene molecules was performed using a stilbene precursor through the process of photocyclization as described previously [1].

### B. Sample Preparation

The fabrication of the Co/Cu(111) substrate involved several steps. The surface of the Cu crystal was first cleaned by repeated cycles of $Ar^+$ sputtering ($p_{\mathrm{Ar}} = 5 \times 10^{-4}$ Pa, 30 min) followed by annealing (850 K, 60 min) to ensure an atomically clean surface. Co bilayer nanoislands were then grown on the surface by in-situ Co deposition at RT using e-beam evaporation from a 99.99% pure Co rod. The deposition rate was 0.2 ML/min and the pressure during deposition was less than $2 \times 10^{-8}$ Pa. The characteristics of the Co bilayer islands, including their shape, density, and cleanliness, were verified by means of topographic STM images. In addition, spin-polarized STM measurements were conducted to confirm the presence of well-defined out-of-plane magnetization of the islands. The substrate was subsequently transferred to a separate chamber for molecular deposition. A racemic powder of [7]H molecules was sublimed from a glass crucible heated to a temperature of 400 K, and the substrate was exposed to the molecular vapor for a duration of less than one minute [2]. The sample was then immediately transferred to the STM chamber without vacuum break and cooled to 5 K for subsequent STM measurements under a pressure of $10^{-9}$ Pa.

### C. STM/STS Measurements

For STM/STS measurements, electrochemically etched polycrystalline tungsten (W) tips were used. If needed, short bias pulses were applied to achieve high spatial resolution. To

obtain magnetic contrast, the W tip is functionalized by bringing it into and out of mechanical contact with a remote Co nanoisland at enhanced bias voltage to transfer Co atoms from the island to the tip apex. This functionalization procedure was performed repeatedly until a $dI/dV$ map was obtained that showed magnetic contrast on Co nanoislands, which served as confirmation of the tip's capability to detect spin polarization of the tunneling current in the direction perpendicular to the substrate.

Four different modes of STM operation are used to address structural, electronic, magnetic, and transport properties of the samples: (i) In constant-current mode, the tip follows an isosurface of the integrated local density of states (LDOS) above the surface. A bias voltage $V_{\mathrm{bias}}$ was applied to the sample, and the height corrections made by the STM feedback loop to regulate the tunneling current to the constant setpoint current $I_{\mathrm{t}}$ were recorded while scanning the surface point-by-point. The recorded data can be interpreted as the topography of the sample. (ii) Differential conductance ($dI/dV$) maps were obtained simultaneously with a constant-current topographic image, i.e., with the feedback loop closed. To extract the $dI/dV$ signal, the DC bias voltage $V_{\mathrm{bias}}$ is superimposed with a small sinusoidal modulation with an rms amplitude of $V_{\mathrm{mod}} = 20\,\mathrm{mV}$ and a frequency of $f_{\mathrm{mod}} = 752\,\mathrm{Hz}$. The resulting modulation of the tunneling current at $f_{\mathrm{mod}}$ is detected with a lock-in amplifier and recorded as a function of the lateral tip position during a scan in a second data channel. $dI/dV$ maps represent to a good approximation the spatial variations of the LDOS above the sample at the energy given by $eV_{\mathrm{bias}}$, where $V_{\mathrm{bias}} = 0$ corresponds to the Fermi energy. (iii) For constant-height STM images, the feedback loop was deactivated and the STM tip was scanned over the sample surface at a fixed height $z_{\mathrm{Co}}$ above the Co surface. The tunneling current flowing due to the applied bias voltage $V_{\mathrm{bias}}$ is recorded as a function of lateral tip position. Setting and keeping constant $z_{\mathrm{Co}}$ with the feedback loop disabled is critical for this type of measurement, since a change of the tip-surface distance by one Ångström leads to a variation of the tunneling current by about one order of magnitude [3]. Therefore, the inclination of the Co surface is first determined from a constant-current image and then used to align the scanning plane of the constant-height measurement coplanar with the Co surface. The height $z_{\mathrm{Co}}$ for a constant-height measurement is set by the bias voltage $V_{\mathrm{bias}}$ and setpoint current $I_{\mathrm{t}}$ applied before switching off the feedback loop and the subsequent retraction of the tip by $\Delta z_0$. The latter is needed to keep the current amplitude within the range of the pre-amplifier (1 pA to 3.3 nA) throughout the constant-height scan.

(iv) For current-voltage ($I - V$) spectra, the tip is moved to the sample spot of interest and the vertical position is stabilized by applying $V_{\mathrm{stab}} = 2\,\mathrm{V}$ with the activated feedback loop regulating the tunneling current to the setpoint current $I_{\mathrm{stab}} = 800\,\mathrm{pA}$ for Figures 2 and 3 of the main text and $I_{\mathrm{stab}} = 500\,\mathrm{pA}$ for Figure 4 of the main text. Then, the feedback loop is deactivated, i.e., the tip height is fixed, and the $V_{\mathrm{bias}}$ is swept in the range from $-1$ to $+1\,V$ and the resulting tunneling current is recorded. The bias sweep is repeated five times to improve the signal-to-noise ratio. The standard error of this averaging is displayed as light colored area in Figures 3a,b and 4b of the main text and is used to calculate the errors of the asymmetries MChA and EMA in Figures 3c and d of the main text. An $I - V$ spectrum obtained in this manner represents, to a good approximation, the energy-dependent integrated LDOS at the fixed position of the tip above the sample surface, where $V_{\mathrm{bias}} = 0$ corresponds to the Fermi energy.

## S2. MAGNETIC SENSITIVITY OF THE STM TIP

Supporting Figure S1a shows a $dI/dV$ map with an extended scanning area that includes the scan area shown in Figures 2b. This $dI/dV$ map was obtained using a Co-functionalized STM tip, which has out-of-plane magnetic sensitivity. This sensitivity is highlighted by the different $dI/dV$ contrast of the two Co islands framed by dashed and dotted rectangles, which is due to their opposite out-of-plane magnetizations. To eliminate the out-of-plane magnetic sensitivity of the tip, it was re-functionalized over a remote bare Cu area by removing the Co atoms from the apex of the W tip. A subsequent $dI/dV$ map measured with the newly Cu-functionalized tip but otherwise identical scanning parameters as in Supporting Figure S1a is displayed in Supporting Figure S1b. The absence of contrast between the islands, including that between the dashed and dotted framed islands, confirms that the tip is no longer sensitive to the magnetization of the out-of-plane magnetized Co islands.

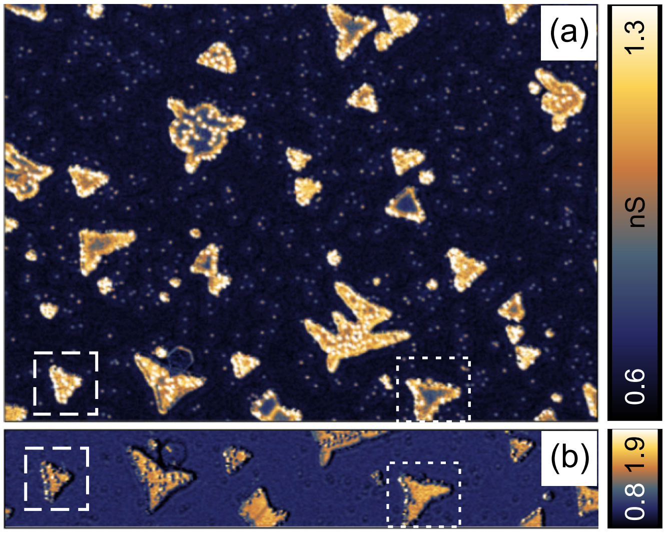


FIG. S1. $dI/dV$ maps with magnetic and non-magnetic tip. (a) The $dI/dV$ map obtained using a Co-functionalized (magnetic) tip demonstrates magnetic contrast between Co nanoislands with opposite perpendicular magnetization, e.g., the islands framed by dashed and dotted rectangles. (b) The same scan area as in (a) was again imaged with the newly functionalized (nonmagnetic) W tip, and no contrast is seen between the two selected islands. This confirms that the tip is no longer sensitive to the out-of-plane magnetization of the Co islands ($V_{\text{bias}} = -600\,\text{mV}$, $I_{\text{t}} = 550\,\text{pA}$, $V_{\text{mod}} = 20\,\text{mV}$, $f_{\text{mod}} = 752\,\text{Hz}$, $5\,\text{K}$).

## S3. SINGLE-MOLECULE $I - V$ SPECTRA

Supporting Figures S2a and c present the single-molecule $I - V$ spectra of five *(M)*-[7]H and *(P)*-[7]H molecules each, located on the dotted framed Co island exhibiting dark $dI/dV$ contrast in Figure 2b of the main text or in Supporting Figure S1a. Similarly, Supporting Figures S2b and d show single-molecule $I - V$ spectra of five other *(M)*-[7]H and *(P)*-[7]H molecules each, located on the Co island exhibiting bright $dI/dV$ contrast in Figure 2b of the main text or in Supporting Figure S1a. After detecting the island magnetization directions using $dI/dV$ maps and before recording the the singe-molecule $I - V$ spectra, the STM tip was re-functionalized in a remote Cu area to obtain a non-magnetic tip insensitive to the spin polarization of the tunneling current (see Supporting Section S2). For each molecule, the tip was positioned above the highest part of the molecule, and after stabilizing the vertical tip position at $V_{\text{stab}} = 2\,\text{V}$ and $I_{\text{stab}} = 800\,\text{pA}$, five consecutive spectra were acquired to enhance signal-to-noise ratios (see Supporting Section S1). The average spectrum for each individual molecule is plotted as dark red or green curve, while the light colored area around the averaged spectrum indicates the standard error associated with the spread of the repeated bias sweeps. In a next step, the five single-molecule spectra for each combination of handedness and island magnetization direction were averaged and plotted in Supporting Figures S2e and f. In these plots, the light colored areas indicate the standard errors due to the averaging over five individual molecules.

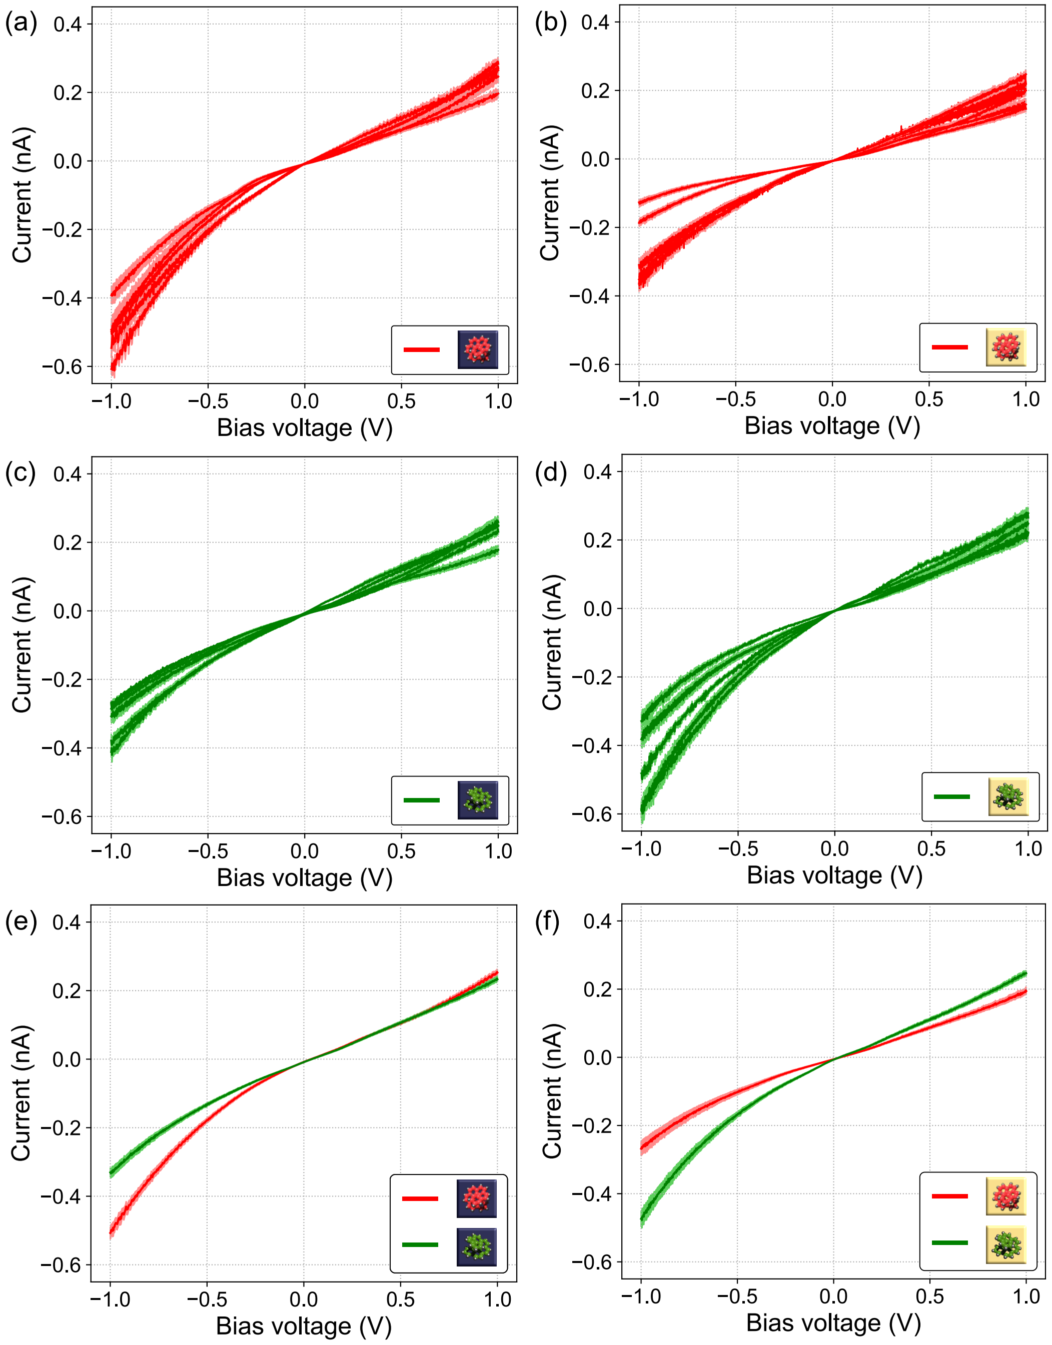


FIG. S2. $I-V$ spectra of molecules adsorbed on two oppositely magnetized Co islands. (a) and (c) Five single-molecule spectra of individual *(M)*-[7]H and *(P)*-[7]H molecules on the dark island, respectively. (b) and (d) Five single-molecule spectra of individual *(M)*-[7]H and *(P)*-[7]H molecules on the bright island, respectively. (e) and (f) Averaged spectra of the five molecules with the same handedness on dark and bright islands, respectively. All $I-V$ spectra were obtained with a non-magnetic STM tip ($V_{\mathrm{stab}} = 2\,\mathrm{V}$ and $I_{\mathrm{stab}} = 800\,\mathrm{pA}$). The dark curves represent the averaged $I-V$ spectra, while the light-colored regions indicate the calculated standard errors.

## S4. REVERSING THE MAGNETIZATION DIRECTION OF THE STM TIP

Supporting Figure S3a shows a $dI/dV$ map featuring [7]H-decorated Co nanoislands on Cu(111). The island framed by the dashed rectangle hosts the molecules shown in the inset of Figure 3a of the main text. The area in the dotted frame is displayed at higher resolution in Supporting Figure S3b. This data was recorded using a Co-functionalized STM tip, referred to in the main text as the first magnetic tip configuration. As observed in Supporting Figure S3b, the islands in the upper left corner of the image exhibit dark $dI/dV$ contrast, whereas the islands in the lower right show bright $dI/dV$ contrast due to their different perpendicular magnetization directions.

After acquiring this data, the tip was moved to a remote Co island and re-functionalized

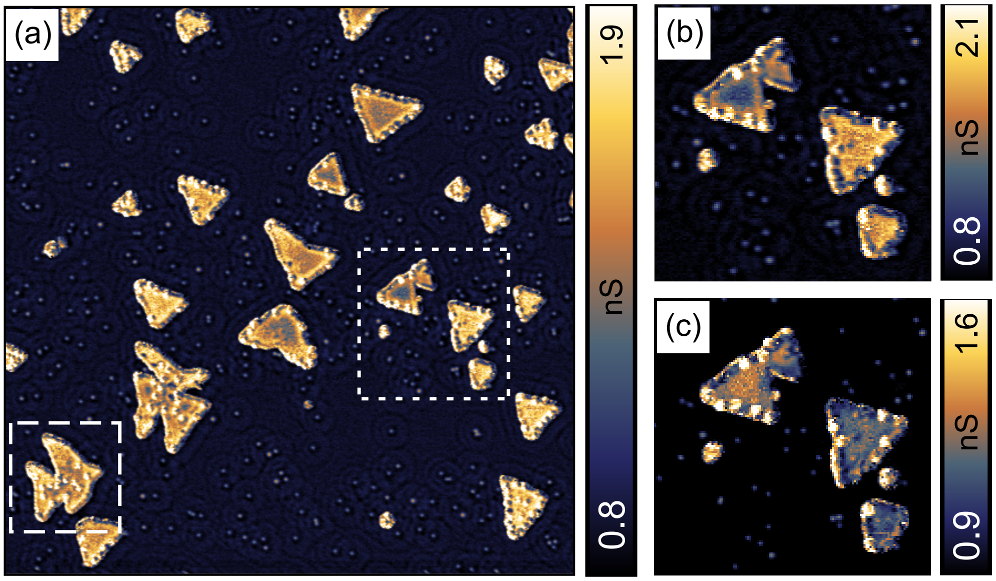


FIG. S3. Reversing the magnetization direction of the STM tip. (a) The $dI/dV$ map, measured with the first magnetic tip configuration, displays magnetic contrast between Co nanoislands with opposite perpendicular magnetization. The island framed by the dashed rectangle contains the molecules depicted in the inset of Figure 3a in the main text. (b) Presents the area indicated by the dotted frame in (a) at a higher resolution. (c) shows the same scan area as in (b) measured with the same scanning parameters, but using a re-functionalized tip referred to as the second magnetic tip configuration. This configuration demonstrates a reversal in the magnetic contrast of the Co nanoislands. ($V_{\mathrm{bias}} = -600\,\mathrm{mV}$, $I_{\mathrm{t}} = 550\,\mathrm{pA}$, $V_{\mathrm{mod}} = 20\,\mathrm{mV}$, $f_{\mathrm{mod}} = 752\,\mathrm{Hz}$, 5 K, Co-functionalized W tip).

to alter the magnetization direction of the tip apex (see Supporting Section S1). After returning to the scan area of Supporting Figure S3b, another $dI/dV$ measurement was performed to assess the magnetic sensitivity of the newly modified tip. This procedure was repeated until the Co nanoislands in Supporting Figure S3b exhibited reversed magnetic $dI/dV$ contrast, as shown in Supporting Figure S3c. In this $dI/dV$ map, the previously dark islands in the upper left corner now appear bright, while the islands in the lower right exhibit dark contrast. This outcome verifies that the tip's out-of-plane magnetic sensitivity is still present, but the magnetization direction of the tip apex has reversed, which is referred to in the main text as the second magnetic tip configuration.

[1] A. Sudhakar and T. J. Katz, Directive effect of bromine on stilbene photocyclizations. An improved synthesis of [7]helicene, Tetrahedron Lett. **27**, 2231 (1986).

[2] M. R. Safari, F. Matthes, K.-H. Ernst, D. E. Bürgler, and C. M. Schneider, Deposition of Chiral Heptahelicene Molecules on Ferromagnetic Co and Fe Thin-Film Substrates, Nanomaterials **12**, 10.3390/nano12193281 (2022).

[3] B. Voigtländer, *Scanning probe microscopy: Atomic force microscopy and scanning tunneling microscopy* (Springer, Berlin, 2015).
